# Supplementary material for: Efficient experimental quantum fingerprinting with wavelength division multiplexing
Source: arXiv:2005.06049 ancillary file (2020-05-12)
Supplement: Supplementary file 1 [file supplementray_v6.pdf]

# Supplementary: Efficient experimental quantum fingerprinting with wavelength division multiplexing

Xiaoqing Zhong,[1,*] Feihu Xu,[2] Hoi-Kwong Lo,[1,3] and Li Qian[3]

[1]*Center for Quantum Information and Quantum Control, Dept. of Physics, University of Toronto, Toronto, Ontario, M5S 1A7, Canada*

[2]*Hefei National Laboratory for Physical Sciences at the Microscale and Department of Modern Physics, University of Science and Technology of China, Hefei 230026, China*

[3]*Center for Quantum Information and Quantum Control, Dept. of Electrical & Computer Engineering, University of Toronto, Toronto, Ontario, M5S 3G4, Canada*

## A. Charlie's decision mechanism

For Charlie to determine whether the inputs of Alice and Bob are equal or not, we adopt the method introduced in Ref. [2] where a threshold value $C_{1,th}$ are needed. When the total counts detected at Charlie's detector $D_1$ is smaller than the threshold $C_{1,th}$, Charlie announces that the inputs $x$ and $y$ are the same. Otherwise, Charlie announces that the inputs are different. The choice of threshold $C_{1,th}$ is dependent on the input size $n$ and the total average photon number $\mu$. The details of this decision mechanism is described as follows.

As described in the main text, ignoring multi-photon contributions, in each detection window, the probabilities for $D_1$ obtaining a click for the equal inputs ($P_E$) and 1-bit different inputs ($P_D$) are:

$$P_E = (1-\nu)(1-e^{-\frac{2\mu\eta}{M}}) + P_{dark} = (1-\nu)(1-e^{-\frac{2k\mu\eta}{m}}) + P_{dark}, \tag{1}$$

$$P_D = (\delta\nu + (1-\delta)(1-\nu))(1-e^{-\frac{2\mu\eta}{M}}) + P_{dark} = (\delta\nu + (1-\delta)(1-\nu))(1-e^{-\frac{2k\mu\eta}{m}}) + P_{dark}. \tag{2}$$

In the above equations, $M$ is the total number of pulses sent from Alice/Bob to Charlie and equals to

$$M = \frac{n/c}{k} = \frac{m}{k}. \tag{3}$$

$n$ is the length of input strings, $c$ is the code rate of an error correction code (ECC) and $m$ is the length of codeword. $k$ is the total number of wavelength channels. $\nu$ is the interference visibility. $\eta$ is the overall transmittance, which is used to include the loss of the optical channel and the detector efficiency in practical demonstration. $\delta$ is the Hamming distance of ECC which defines the minimum distance between two different codewords. $P_{dark}$ is the dark count probability of the single photon detector (SPD). Since each detection event is independent, the distributions of the total counts registered at $D_1$ f or the equal and different inputs cases can be modeled as the binomial distributions $B(M, P_E)$ and $B(M, P_D)$ respectively. As indicated, in each detection window, there are $k$ pairs of coherent states at different wavelengths interfering simultaneously. Here we ignore any possible cross talk between adjacent channels and assume that the interference of states in each wavelength channel is independent. The distributions of the total counts at $D_1$ depend on the total number of pulses $M$ sent to Charlie and the total mean photon number $\mu$. Moreover, for the same $M$ and $\mu$, the distributions of the total counts at $D_1$ for the equal and different inputs cases are different, leading to different expectation values,

$$\begin{aligned} \lambda_E &= M \times P_E \\ \lambda_D &= M \times P_D. \end{aligned} \tag{4}$$

In the coherent fingerprinting scheme, the size of the inputs of interest is very large ($> 10^5$) and the detection probabilities $P_E$ and $P_D$ are always on the same order as the dark count probability ($10^{-6}$). Therefore, the above binomial distributions in this case are well described by the Poisson distributions $Poi(\lambda_E)$ and $Poi(\lambda_D)$. Fig. (1) shows an example of the distributions of the total counts at $D_1$ for both the same inputs case (blue curve) and different inputs (red curve) case. As indicated, the probability distributions for the two cases are away from each other. For most of the time, the total counts for different inputs case $C_{1,D}$ are larger than the counts for equal inputs case $C_{1,E}$. Therefore, Charlie could choose a threshold total counts $C_{1,th}$ and compare $C_{1,th}$ with the detected photon counts at $D_1$. If the number of the detected counts is smaller (larger) than $C_{1,th}$, Charlie concludes that Alice and Bob have the same (different) inputs. The errors exist when $C_{1,E}$ is actually larger than the threshold, or $C_{1,D}$ is smaller than the threshold. The error probability for Charlie's decision is then defined by

$$P_{error} = max[P_r(C_{1,E} > C_{1,th}), P_r(C_{1,D} < C_{1,th})]. \tag{5}$$

As long as $P_{error}$ is smaller than a tolerable error probability $\epsilon$, Charlie's conclusion is acceptable.

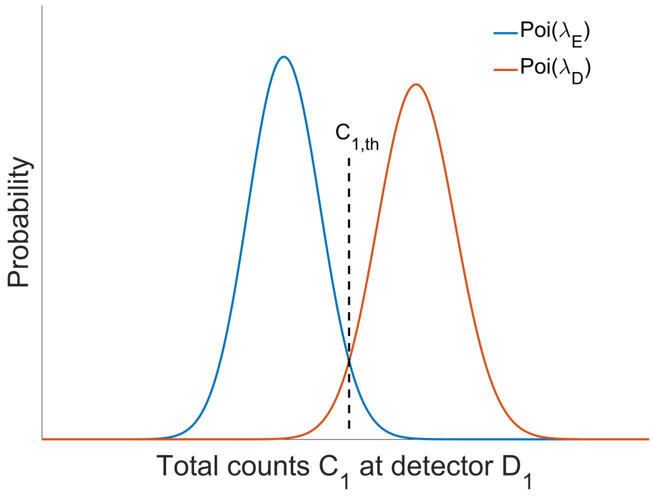


FIG. 1: Probability distribution of the total counts at detector $D_1$ for the equal inputs case (blue curve) and different inputs case (red curve). In this figure, the total number of pulses $M$ is $5 \times 10^8$. $\delta$ and $\nu$ in Eq.(1) and Eq.(2) are 0.22 and 97% respectively. The detector's dark count probability is $10^{-6}/ns$ and $\eta = 0.2$ is considered as the detector efficiency (20%). The average photon number $\mu$ is 1000. Note that this figure just shows an example of the probability distributions. Hence the value of $\mu$ is not necessarily optimal and the corresponding error probability might be large.

### B. Upper bound of error probability

In this section, an upper bound of Charlie's error probability is discussed. For Poisson distributions, the Chernoff bound provides the upper bounds of probabilities $P_r(C_{1,E} > C_{1,th})$ and $P_r(C_{1,D} < C_{1,th})$ in Eq.(5) as

$$\begin{aligned} P_r(C_{1,E} > C_{1,th}) &< \frac{e^{-\lambda_E}(e\lambda_E)^{C_{1,th}}}{C_{1,th}{}^{C_{1,th}}} \\ P_r(C_{1,D} < C_{1,th}) &< \frac{e^{-\lambda_D}(e\lambda_D)^{C_{1,th}}}{C_{1,th}{}^{C_{1,th}}}, \end{aligned} \tag{6}$$

as long as the threshold $C_{1,th}$ is chosen to satisfy

$$\lambda_E < C_{1,th} < \lambda_D. \tag{7}$$

Moreover, if threshold $C_{1,th}$ is the crosspoint of the two distributions $Poi(\lambda_E)$ and $Poi(\lambda_D)$, i.e.

$$Poi(C_{1,th}; \lambda_E) = Poi(C_{1,th}; \lambda_D), \tag{8}$$

then the upper bounds for the error probabilities $P_r(C_{1,E} > C_{1,th})$ and $P_r(C_{1,D} < C_{1,th})$ are the same. In this case,

$$C_{1,th} = \frac{\lambda_E - \lambda_D}{log_e(\lambda_E/\lambda_D)} \tag{9}$$

and the upper bound for Charlie's error probability is

$$P_{error} < P_{upper} = \frac{e^{-\lambda_E}(e\lambda_E)^{C_{1,th}}}{C_{1,th}{}^{C_{1,th}}}. \tag{10}$$

### C. Optimization of $\mu$

As indicated by the above equations, the error probability depends on the total number of pulses $M$ and the total mean photon number $\mu$. If $M$ and $\mu$ are known, one can use Eq. (5) to search a optimal threshold $C_{1,th}$ (between $\lambda_E$ and $\lambda_D$) which gives the minimum error probability. As shown in Eq. (3), for a given system (ECC and $K$ are fixed), $M$ is only determined by the input

size $n$. Now, the question is how to determine the average photon number $\mu$ for each value of $M$, as well as its corresponding optimal threshold $C_{1,th}$. On one hand, $\mu$ should be large enough such that the detection probabilities ($P_E$ and $P_D$) are not dominated by $P_{dark}$ and the error probability is below $\epsilon$. On the other hand, since the amount of communication required is $Q = O(\mu log_2 n)$, $\mu$ should be as small as possible. Therefore, there is a tradeoff between $P_error$ and the minimum amount of communication $Q$. In our work, $C_{1,th}$ is given by Eq. (9) which is a function of $M$ and $\mu$. Then for each value of $M$, the optimization of $\mu$ can be done by searching the **minimum** value of $\mu$ and the corresponding $C_{1,th}$, which satisfies the error probability condition, i.e. $P_{error} < \epsilon$. As shown in Fig. (2a), the solid curves are the error probability $P_{error}$ given in Eq. (5) as a function of the total mean photon number $\mu$ for three different values of $M$ ($5 \times 10^6, 5 \times 10^7, 5 \times 10^8$). The optimal $\mu$ for different $M$ is indicated by the yellow circle, the corresponding $P_{error}$ of which is just below the tolerable error probability $\epsilon = 10^{-5}$ (black solid line).

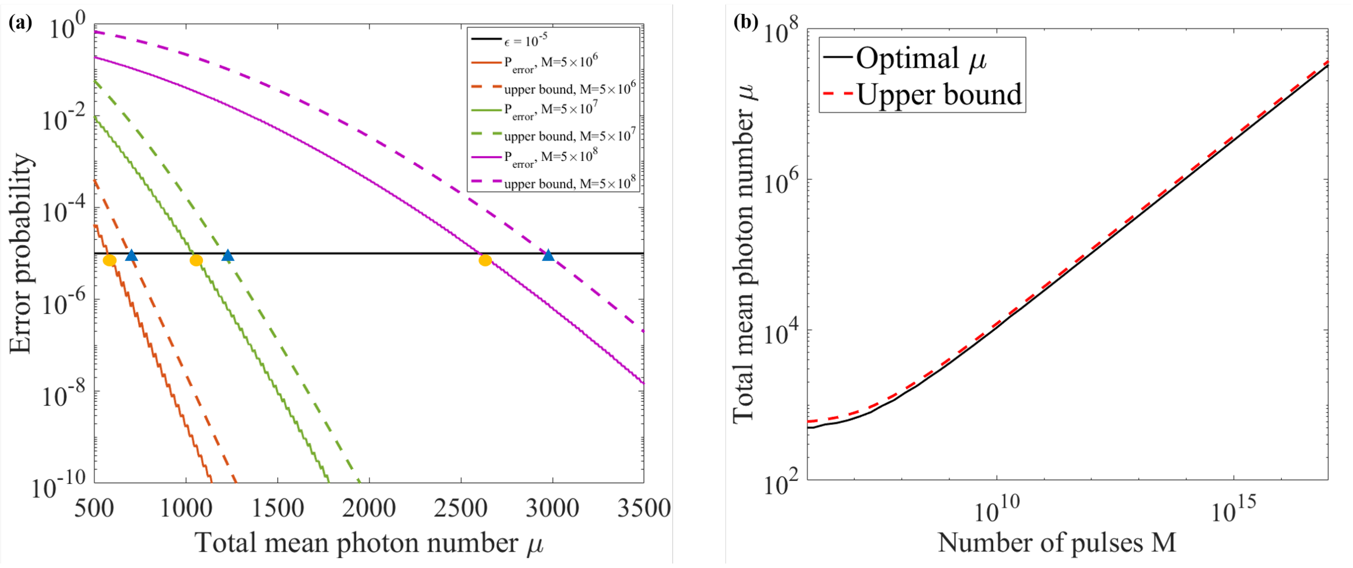


FIG. 2: **(a)** Log-log plot of error probability as a function of total average photon number $\mu$. Three different values of $M$ (total number of pulses) are tested, that are $5 \times 10^6, 5 \times 10^7, 5 \times 10^8$. The solid curves indicate the error probability calculated based on Eq. (5) and Eq. (9). The yellow circles are the optimal $\mu$ chosen for different sizes of $M$. The dash curves are the upper bounds $P_{upper}$ in Eq. (10) for different sizes of $M$. The blue triangles are the values of $\mu$ that satisfy Eq. (11). **(b)**: Log-log plot of total mean photon number $\mu$ as a function of the number of pulses $M$ sent from Alice/Bob to Charlie. The black solid curve is the optimal $\mu$ searched for each $M$. The red dash curve is the upper bound of $\mu$ calculated from Eq. (11).

Or, more simply, we don't have to search the optimal $\mu$ one by one. We can fix the upper bound of $P_{error}$ to be equal to $\epsilon$, i.e.

$$P_{upper} = \frac{e^{-\lambda_E}(e\lambda_E)^{C_{1,th}}}{{C_{1,th}}^{C_{1,th}}} = \epsilon = 10^{-5}. \tag{11}$$

Then for each given $M$, one can directly calculate $\mu$ from the above equation. In this case, $P_{error}$ can be always smaller than $\epsilon$. In Fig. (2a), the dash curves are the upper bounds of $P_{error}$ as a function of $\mu$ for different sizes of $M$. The calculated $\mu$ based on Eq. (11) for different $M$ is indicated by the blue triangle. As shown in Fig. (2a), this calculated $\mu$ is actually larger than the optimal $\mu$. For a small size of $M$, as in our experiment, searching the optimal $\mu$ can be done very quickly. For a very large size of $M$, searching optimal $\mu$ might be time consuming, while directly calculating $\mu$ is very straightforward. Note that this calculated $\mu$ is actually the upper bound, as indicated in Fig. (2b). The black solid curve is the optimal $\mu$ as a function of $M$ and the red dash curve is the upper bound of $\mu$ calculated based on Eq. (11). Since $Q = O(\mu log_2 n)$, for a given $n$, this upper bound of $\mu$ also gives the upper bound of the amount of communication in our WDM-CQF protocol. We remark that this upper bound might not be precise but fair enough as long as the Poisson distribution approximation used in ”section A” is valid. The strict proof of this conclusion is out of the scope our paper.

### D. Validity of simultaneous interference and detection of k pairs of wavelength components

The advantage of transmitting less amount of information in our WDM-CQF protocol benefits from the shared detecting system for the $k$ pair of wavelength components. As shown in Fig. (2b), the total average photon number $\mu$ is a function of

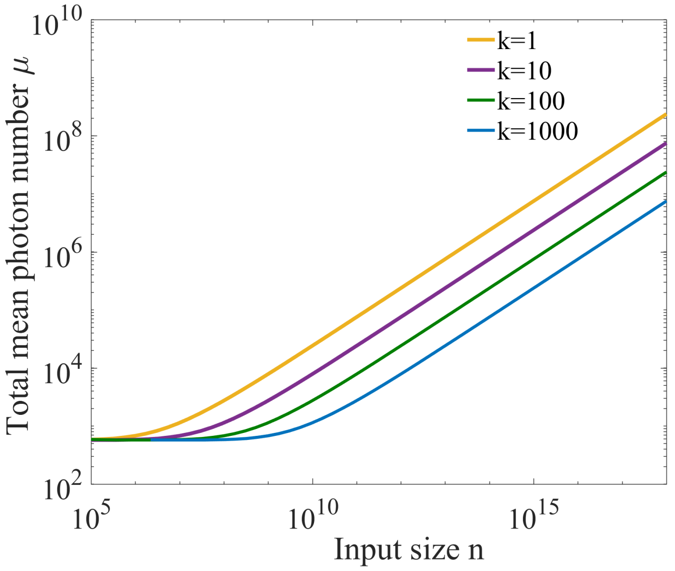


FIG. 3: Log-log plot of the total average photon number $\mu$ required by the WDM-CQF protocol with different wavelength channels as a function of the input size $n$. When $k = 1$, the scheme becomes to the original CQF scheme. Note that in this figure, $\mu$ is not the optimal, but satisfies the condition in Eq. (11), i.e., the upper bound of the error probability equal the tolerable error probability $\epsilon$.

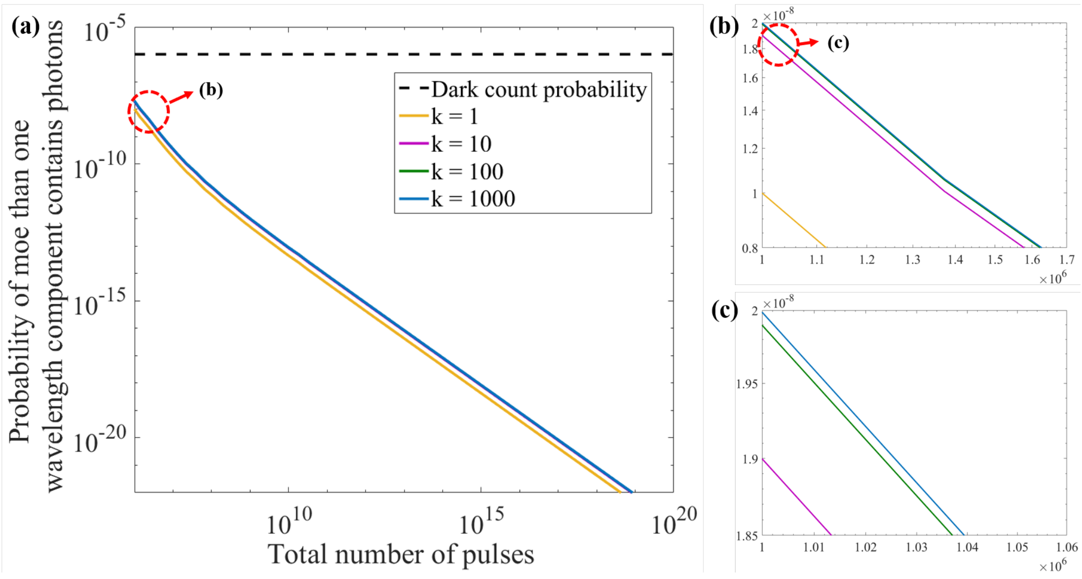


FIG. 4: **(a)**: Probability of the case that, for each pair of pulses arriving at Charlie's station, more than one wavelength component contains photons as a function of $M$. Black dash line is the dark count probability ($10^{-6}$) considered in our scheme. **(b)**: An enlarged figure of the red circle area in (a). **(c)**: An enlarged figure of the red circle area in (b). Different numbers of wavelength channels are tested ($k \in \{1, 10, 100, 1000\}$).

the total number of pulses $M$ sent out by Alice and Bob. In other words, as long as $M$ is fixed, the average photon number in each wavelength composite pulse is fixed no matter how many wavelength components ($k$) it contains. For a fixed input size $n$, if more wavelength channels $k$ are used, the number of pulses sent from Alice/Bob to Charlie $M$ is fewer ($M = n/(ck)$). Consequently, the less $\mu$ is required and the total amount of communication is reduced. Fig. (3) shows the total average photon number $\mu$ required as a function of input size $n$ for different value of $k$. It is clear that for large input size, the more wavelength channels are applied, the smaller value of mean photon number is required.

In Eq.(1) and Eq.(2), the $k$ pair of wavelength components interfere simultaneously and are detected by a single pair of SPDs. As mentioned before, we assume that only the states in the same wavelength channel would interfere with each other. In fact, in coherent quantum fingerprinting protocol, to minimize the amount of communication, $\mu$ is always chosen to be so small that

most of the pulses arriving at Charlie's station are vacuum. At Charlie's station, before the interference, the probabilities of each wavelength component being vacuum or having photons are

$$P_{vac} = e^{-\frac{\mu\eta}{m}} \tag{12}$$

and $(1 - P_{vac})$ respectively. For each pair of interfering pulses sent out by Alice and Bob, there are in total $2k$ components. Then, the probability that, more than one component, either from Alice or Bob, carries photons when arriving at Charlie's station is given by

$$P = 1 - {P_{vca}}^{2k} - 2k \times (1 - P_{vac}) \times {P_{vac}}^{2k-1}. \tag{13}$$

In Fig. (4), we plot out the probability $P$ as a function of the total number of pulses $M$. As shown in Fig. (4), for different values of $k$, this probability is always orders of magnitude smaller than the dark count probability, which is around $10^{-6}$ in our scheme, especially for large $M$. As indicated in the enlarged Fig. (4b) and Fig. (4c), when $k$ increases from $k = 1$ to $k = 1000$, the increase of this probability is very small. That is to say, even for large $k$, we could ignore the case that more than one wavelength component carries photons when each pair of pulses arrive at Charlie's beam spiltter. In this case, even there are $k$ pairs of wavelength components interfere simultaneously, at most, only one of them has photons and can make a contribution to the detection event. Moreover, the information about which wavelength component has a photon is not irrelevant, since Charlie's decision is only determined by the total number of counts at detector $D_1$ as discussed in "section B". Therefore, in our scheme, de-multiplexing is not needed on Charlie's station and one pair of SPDs is adequate.

We remark that when $M$ is relatively small (smaller than $10^5$), the above discussion would not be valid any more, since the probability of the interfering pulses having more than one non-empty wavelength component would be too large to be ignored. Therefore, for WDM-CQF system with different wavelength channels, the smallest size of input of interest is different. To benefit from applying large number of wavelength channels, the input size should also be large.

---

* Electronic address: xzhong@physics.utoronto.ca

[1] Arrazola J. M. and Lütkenhaus N.. Quantum fingerprinting with coherent states and a constant mean number of photons. *Physical Review A*, 89(6), 062305 (2014).

[2] Xu F., Arrazola J.M., Wei K., Wang W., Palacios-Avila P., Feng C., Sajeed S., Lütkenhaus N. and Lo H.-K.. Experimental quantum fingerprinting with weak coherent pulses. *Nature Communications*, 6, 8735 (2015).
